# Supplementary material for: Slip behavior during pressure driven flow of Laponite suspension
Source: arXiv:2105.02025 source file (2021-05-05)
Supplement: Supplementary file 1 [file supplementary_material.pdf]

**Supplementary Material**

The details about the experimental system and the methodology to support the main manuscript text content are provided over here.

## I. Pulsation Dampener

The inherent design and operation of the peristaltic pump causes pressure fluctuations in the flowing fluid. These fluctuations superimpose on the actual pressure drop experienced by the fluid flowing through the cylindrical tube. To minimize these fluctuations, the outflow from the peristaltic pump is passed through a customized dampener, the schematic for which is shown below. It comprises of a chamber (diameter: 1 cm, height: 1.5 cm & partition width: 0.2 cm) made from polypropylene and fixed with an inlet and an outlet. The fluid from the peristaltic pump flows in to the chamber which is closed from above with a silicone rubber sheet. The pressure fluctuations in the entering fluid get damped due to the presence of rubber sheet and the chamber capacity (150 x $10^{-3}$ $cm^3$). This fluid, with minimzed pressure fluctuations, then flows from the chamber towards the cylindrical tube.

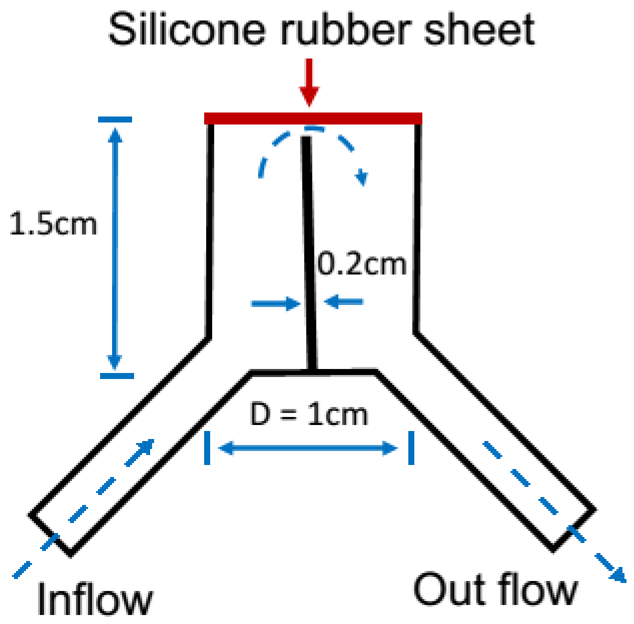


Figure 1. Schematic of the pulsation dampener.

The performance of the dampener was tested by using PDMS fluid (viscosity: $10^{-3}$ Pa s and density: 0.98 g/$cm^3$). The variation of the measured pressure across the length of the cylindrical tube is shown in figure 2 below. As clearly observed, the fluctuations in the measured pressure are in the range of 6 – 8 kPa during the pumping of PDMS (blue line on figure 2 a and b). These fluctuations are reduced significantly (in the range: 0.1 kPa) after PDMS is passed through the dampener (as shown in figure 2 a and b with black line)

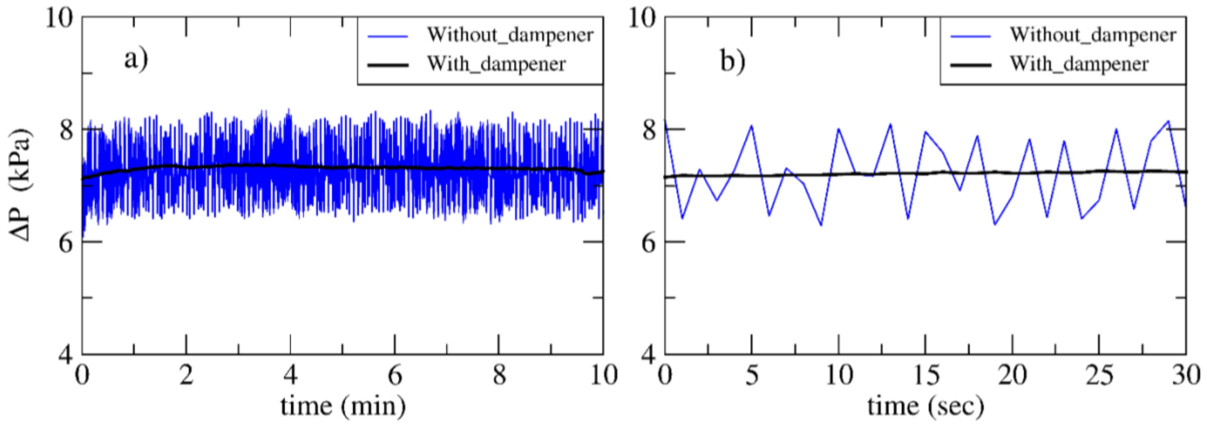


Figure 2. Variation of pressure difference of flowing PDMS through cylindrical tube (D = 0.1cm and L = 24 cm) at a fixed flow rate (0.42 $cm^3$/min) with and without use of the dampener connected upstream. (a) Time dependence over 10 minutes (b) Magnified view showing the effect of the dampener. The peristaltic pump has a period of about 17 s.

## II. In-line fluid mixer

During the experiment, either a stream of salt (NaCl) or water solution is continuously pulsed for a fixed duration into the flowing Laponite suspension. The Laponite-salt or Laponite-water fluid is, then, passed through a customized, in-house mixer before entering the cylindrical tube. The mixer comprises alternate stretched and compressed tube cross-section, respectively leading to flow expansion and contraction. The schematic of the mixer is shown in figure 3. This design has been analyzed in detail in the literature [1] and has been shown to offer efficient mixing by chaotic advection.

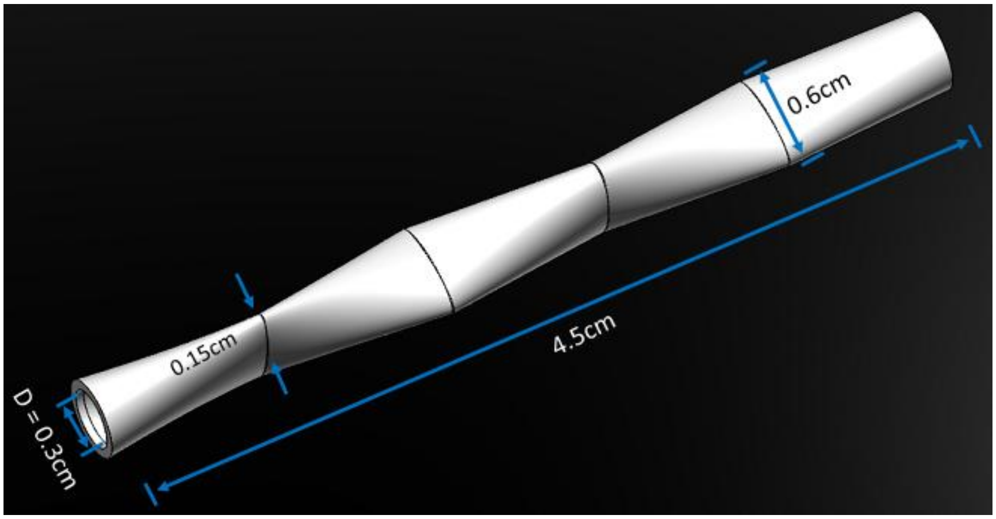


Figure 3. Schematic of inline static mixer.

To verify the occurrence of mixing, a test experiment was conducted by adding a red dye to the pulsed stream of salt solution. The outflow from the mixer was released to atmosphere through a 0.3 cm diameter and 3 cm length tubing. The snapshot taken during the outflow from the tubing

connected to the mixer is shown in figure 4. The uniformity of the color along the tubing length and cross-section is suggestive of very good mixing.

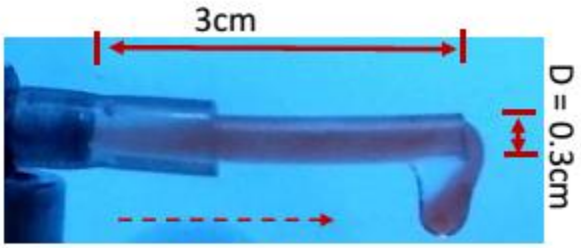


Figure 4. Digital image (snapshot) showing outflow of the mixture of Laponite suspension and (red color) dyed salt solution taken at downstream of the pressure measurement point.

### III. Effect of shear mixing on state of the suspension (Flow rate measurements)

All the experiments are carried under constant peristaltic pumping conditions. Laponite dispersion ages with time and this results in significant change in the viscosity. It is important that the Laponite dispersion that is pumped out from the mixing vessel does not change with time. Our experiment is designed with this in mind: dry Laponite powder and water are added to the mixing vessel where they are subjected to high speed shear mixing. We use a peristaltic pump to flow the dispersion from this vessel and monitor the flow rate for time scales of several hours, comparable to the experimental time scales. Here, the dispersion is not pumped through long tubes as in the reported experiments – rather, we measure the flow rate at the outlet of the tubing just as it emerges from the peristaltic pump. We observe that there is no systematic variation in the flow rate over this time frame, suggesting that the mixing protocol employed in this work affords Laponite dispersion with a well-defined time-independent microstructure. Laponite platelets in the dispersion interact and form an aggregated microstructure as they are pumped through the pipes during the experiment.

### IV. Flow visualization

To visualize the flow characteristics, a small amount of tracer particles (glass beads of diameter 50 microns obtained from Potters Inc.) were inserted in the flowing suspension just before the tube entrance for a small duration overlapping the salt solution pulse. The particles were observed to remain suspended in the flowing stream throughout the length of the tube given the high viscosity of the suspension. A green laser sheet (wavelength 532 nm and thickness 100 microns) was used to illuminate a planar section along the length of the tube of length 3 mm, located 3 cm upstream of the tube exit. The illuminated region in the tube was imaged at 10 frames per second using a digital camera placed orthogonal to the laser sheet plane. Only the upper half of the tube was imaged given the symmetric nature of the flow. The accompanying video (movie.avi) obtained from the image sequence shows a plug-like motion of suspension across the tube radius. The upper edge of the image represents the tube surface while the bottom edge of the image represents the

axis. The bright lines along the image length represent the scatter of the laser sheet from the tube surface and the suspension within.

It is to be noted that while the visualization system was good enough to qualitatively assess the nature of the flow, the image quality, unfortunately, was not good enough to quantitatively characterize the flow behavior accurately, the primary reason being significant scatter from the incident laser sheet.

References


1. Nguyen, N. T. Micromixers: fundamentals, design and fabrication, Elsevier, 2011
